# Supplementary material for: PathAgent: Toward Interpretable Analysis of Whole-slide Pathology Images via Large Language Model-based Agentic Reasoning
Source: arXiv:2511.17052 source file (2025-11-21)
Supplement: Supplementary file 1 [file X_suppl.tex]

\clearpage
\setcounter{page}{1}
% \maketitlesupplementary

\newpage
\twocolumn[{
\begin{center}

    % ---- Supplementary 标题 ----
    {\Large \textbf{\thetitle}}\\[0.5em]
    Supplementary Material\\[1.0em]

    % ---- 第一页大图 ----
    \includegraphics[width=\linewidth]{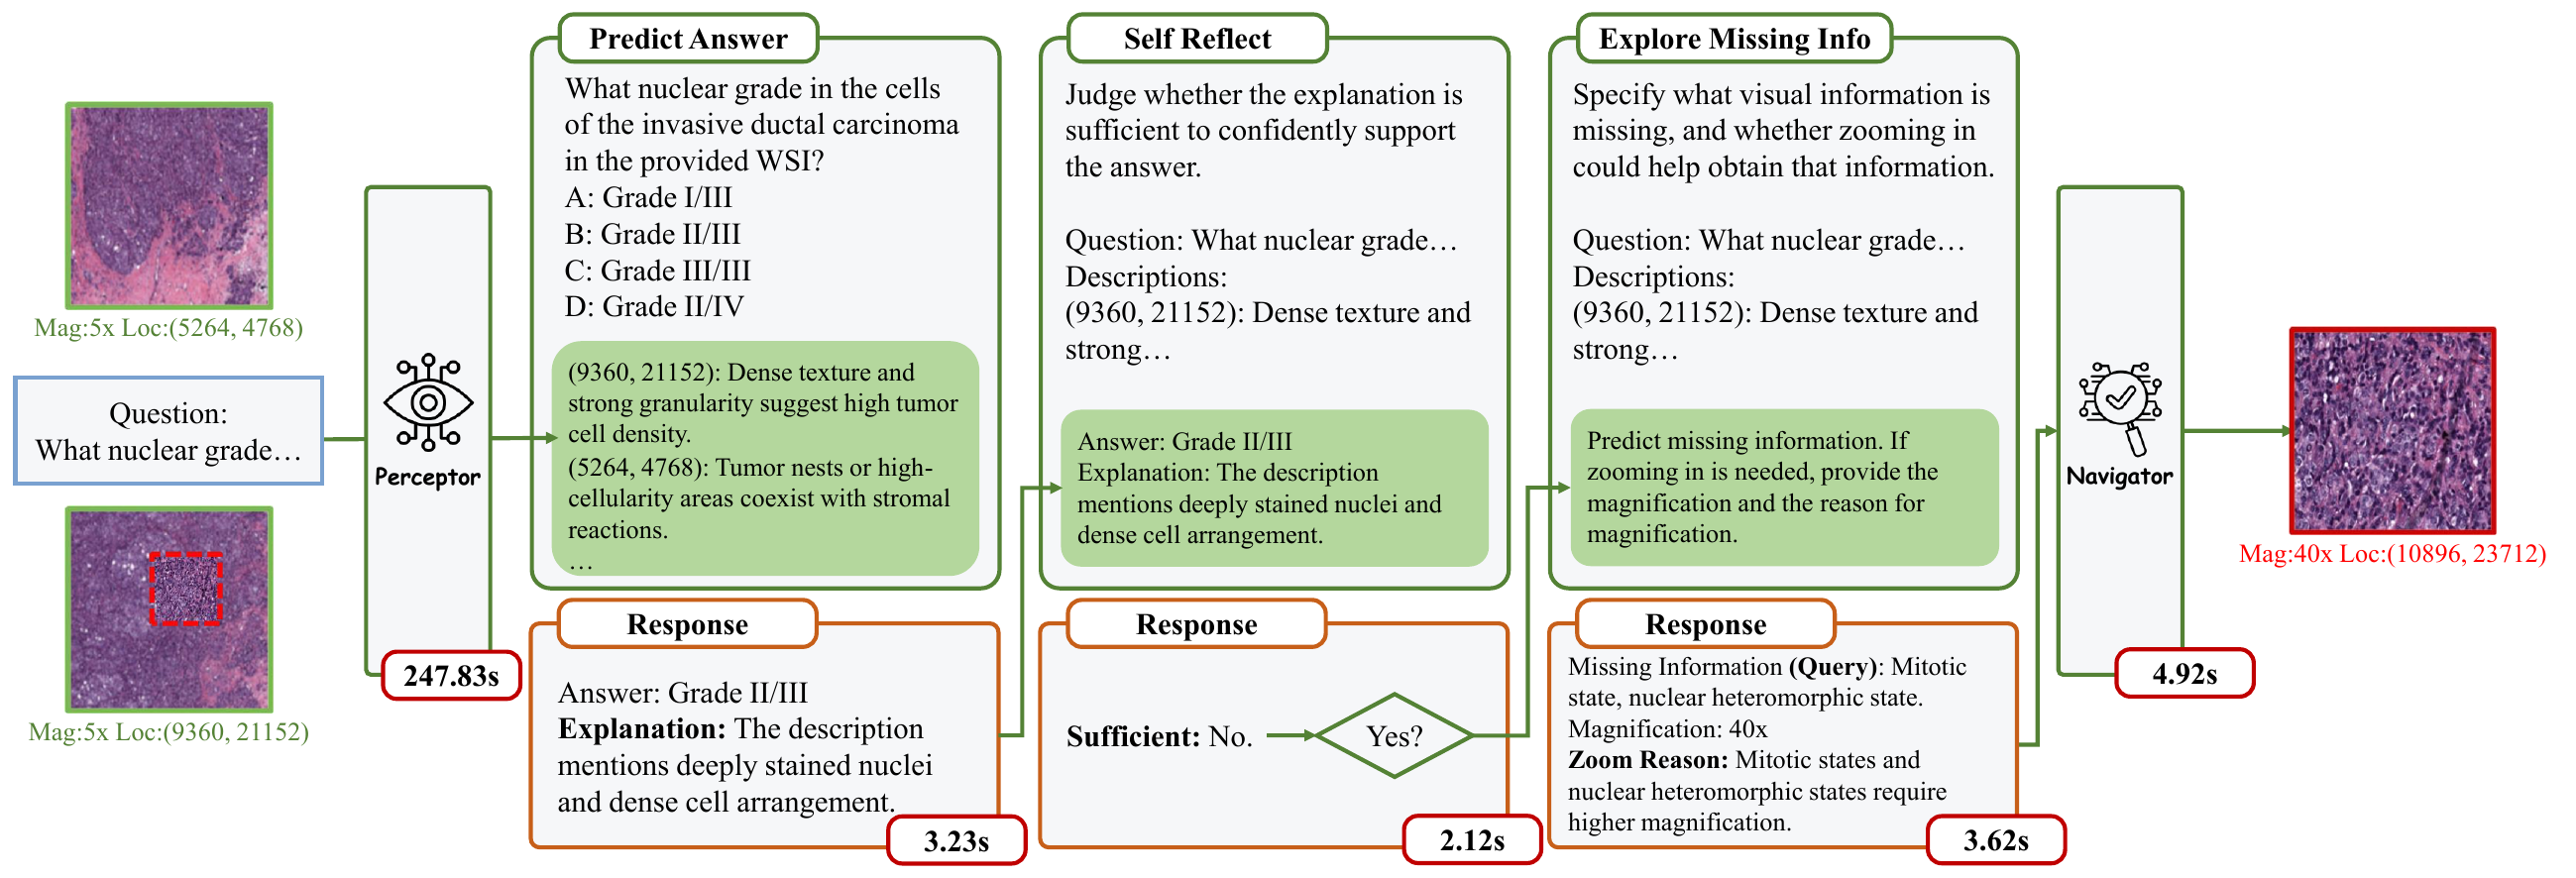}
    \captionof{figure}{
        Inference details of the Executor in PathAgent.
        The Executor executes answer prediction, self-reflection,
        and missing information exploration (if necessary) sequentially,
        providing guidelines for the entire analysis process. 
        The mean time consumption for each stage is shown in the red box below.
    }
    \label{fig:details}

\end{center}
}]

% \twocolumn[{
% \begin{center}
%     \includegraphics[width=\linewidth]{sec/figure/Details.pdf}
%     \captionof{figure}{
%         Inference details of the Executor in PathAgent.
%         The Executor executes answer prediction, self-reflection,
%         and missing information exploration (if necessary) sequentially,
%         providing guidelines for the entire analysis process. 
%         The time consumption for each stage is shown in the red box below.
%     }
%     \label{fig:details}
% \end{center}
% }]

\section{Model Details}
As illustrated in \Cref{tab:capability}, we summarize the capabilities of existing agent systems in comparison to PathAgent. Compared with PathFinder, which only accepts whole-slide images (WSIs), PathAgent supports inputs from both thumbnails and WSIs. Notably, PathAgent is the only agent system that supports human intervention, and we plan to open-source it to further advance research in this area.
% 我们总结了existing agent systems和PathAgent能力上的比较，我们的模型可以接收thumbnails和whole-slide images的输入，而WSI-Agents只支持Thumbnails的输入，PathFinder只支持whole-slide images的输入。此外，仅有PathAgent支持Human intervention，这是PathAgent的一大亮点。PathAgent将会在未来开源。

\Cref{fig:details} illustrates the Multi-Step Reasoning of PathAgent. The Executor receives the generated description from the Perceptor, makes an initial prediction for the answer based on the description, and provides an explanation for its prediction. Then, using the output of the answer prediction, the Executor reflects on whether the explanation is sufficient to support the given answer. If the explanation is sufficient, it indicates that the currently collected evidence adequately answers the question. If it is insufficient to support the given answer, PathAgent needs to further identify what additional information is required to answer the question. In the missing information exploration step, the Executor receives the responses from the first two steps and identifies the missing information required for subsequent analysis. If obtaining the missing information requires magnifying the current images, the Executor also returns the target magnification and the reason for it. It is worth noting that the missing information is used as the text query for retrieving key RoIs with the Navigator.

Specifically, when receiving the question ``What nuclear grade in the cells of the invasive ductal carcinoma in the provided WSI?'' and the corresponding description of the RoIs, the Executor initially answers as Grade II/III. This is because it only receives the description of deeply stained nuclei and dense cell arrangement, visual evidence that supports the Grade II/III answer, but does not rule out the correct option, Grade III/III. Consequently, in the self-reflection stage, the Executor determines that the current information is insufficient to give the correct answer, as both Grade II/III and Grade III/III exhibit deeply stained nuclei and dense cell arrangement. The model then performs missing information exploration, aiming to discover finer morphological characteristics to provide the most comprehensive answer. Therefore, in this stage, the Executor specifies that the mitotic state and nuclear heteromorphic state need to be investigated, and determines that this further information needs to be examined at higher magnification. This guides the Navigator to the $40\times$ patch region to begin the next round of analysis iterations.

We also analyze the time spent at different stages of the entire reasoning process. In this case, the most time-consuming stage is generating descriptions for the most relevant images. In this stage, the Perceptor converts visual information into textual descriptions, which are the source of all diagnostic information. In addition, the Executor's completion of the three steps of Multi-Step Reasoning takes approximately 2-3 seconds. The Navigator's process of using missing information as a query to find new images takes 4.92 seconds.

% 我们还展示了整个推理过程不同阶段的时间消耗，在这个案例中，时间消耗最长的是为最相关的图像生成描述的过程，这一阶段Perceptor将视觉信息转换为文本描述，是所有诊断信息的来源。除此之外，the Executor执行Multi-Step Reasoning的三个步骤用时消耗接近，约为2-3s。Navigator利用Missing Information作为query查找新图像的过程耗时为4.92s。

% \Cref{fig:details}详细描述了Multi-Step Reasoning of PathAgent，the Executor接收来自Perceptor的生成的描述，根据描述初步预测答案并给出相应解释，随后利用第一步answer prediction的输出，重新反思解释是否足以支撑给出的答案，若足以支撑给出的答案，说明目前收集到的证据可以正确回答问题，Multi-Step Reasoning流程结束，若不足以支撑给出的答案，PathAgent需要进一步判断what additional information is needed to answer the question. 在第三步missing information exploration时，the Executor接收到来自前两步的response，并给出missing information用于后续分析，若missing information需要放大当前图像以获取更多信息，the Executor还会返回目标放大倍率和放大的理由。值得注意的是，missing information会被当做后续使用Navigator对key RoIs进行检索的文本query。具体来说，当接收到问题``What nuclear grade in the cells of the invasive ductal carcinoma in the provided WSI?''和patch区域相对应的描述时，the Executor给出初步的答案是Grade II/III，这是因为它只接收到了deeply stained nuclei and dense cell arrangement的描述，这一视觉证据是支撑Grade II/III这一答案的，但是并不能排除正确选项Grade III/III。因此在self-reflection阶段，the Executor判断当前信息不足以给出正确答案，因为Grade II/III和Grade III/III都会呈现出deeply stained nuclei and dense cell arrangement的现象。进而模型执行missing information exploration，旨在发现更细致的morphology characteristic以给出最全面的答案。因此在这一阶段，the Executor给出guidelines that需要检查Mitotic state, nuclear heteromorphic state，并且判断出这些further information需要在更高的倍率下进行进一步检查，由此指导Navigator到40x的patch区域中开始下一轮次的分析迭代。

\begin{table*}[t]
  \caption{A comparison of PathAgent with existing agent systems in computational pathology, where ``All'' in the ``Image type'' column indicates that the model accepts both thumbnails and whole-slide images.}
  \centering
  \resizebox{\textwidth}{!}{
  \begin{tabular}{c|ccccc}
    \toprule
    Method & Type & Training & Image type & Human intervention & Open source  \\ 
    \midrule
    WSI-Agents~\cite{wsi-agents} & Multi-agent collaboration & Training-free & All & Not supported & $\times$  \\
    SlideSeek~\cite{slideseek} & Multi-agent collaboration & Training-need &  All & Not supported & $\times$  \\
    CPathAgent~\cite{CPathAgent} & VLM-based agent & Training-need & All & Not supported & $\times$  \\
    PathFinder~\cite{pathfinder} & Multi-agent collaboration & Training-need & Whole-slide image & Not supported & $\times$  \\
    SmartPath-R1~\cite{SmartPath-R1} & VLM-based agent & Training-need & All &  Not supported  & $\times$ \\
    \rowcolor{gray!20} \textbf{PathAgent} & Multi-agent collaboration & Training-free & All & Supported & \checkmark \\
    \bottomrule
  \end{tabular}
  }
  \label{tab:capability}
\end{table*}

\begin{table*}[t]
  \caption{Comparison of zero-shot visual question answering between our PathAgent and current state-of-the-art methods on PathMMU dataset. The best performance is in \textbf{bold}, while the second-best performance is \underline{underlined}.}
  \centering
  \begin{tabular}{c|cccccc}
    \toprule
    \multirow[c]{2}{*}{Method} & \multicolumn{6}{c}{PathMMU} \\ 
    \cmidrule(lr){2-7}
    % \cline{3-10}
     & PubMed & SocialPath & EduContent & Atlas & PathCLS & Accuracy \\ 
    \midrule
    Qwen3-VL~\cite{Qwen-VL} & 44.63 & 49.12 & 44.31 & 45.88 & 27.67 & 45.82  \\
    GPT-4o~\cite{GPT-4V} & \underline{50.54} & 53.64 & 50.12 & 55.29 & 23.47 & 49.31  \\
    LLaVA-Med~\cite{llava-med} & 27.69 & 27.36 & 27.18 & 30.73 & 20.31 & 26.25  \\
    MedDr~\cite{meddr} & 21.37 & 25.34 & 32.95 & 31.45 & 22.17 & 28.33 \\
    Quilt-LLaVA~\cite{Quilt-llava} & 42.63 & 46.68 & 45.31 & 42.79 & \underline{29.28} & 41.54 \\
    \midrule
    WSI-VQA~\cite{wsi-vqa} & 32.69 & 35.93 & 34.63 & 50.37 & 21.38 & 33.64 \\
    SlideChat~\cite{slidechat} & 50.49 & \underline{55.64} & \underline{50.33} & \underline{56.97} & 25.31 & \underline{50.82} \\
    WSI-LLaVA~\cite{wsi-llava} & 47.35 & 53.26 & 47.22 & 53.81 & 24.87 & 49.57 \\
    TITAN~\cite{titan} & 38.29 & 40.49 & 30.48 & 33.24 & 21.49 & 32.77 \\
    \rowcolor{gray!20} \textbf{PathAgent} & \textbf{51.26} & \textbf{57.71} & \textbf{51.46} & \textbf{59.39} & \textbf{48.53} & \textbf{53.19} \\
    \bottomrule
  \end{tabular}
  \label{tab:zero-shot on PathMMU}
\end{table*}

\begin{figure*}[t]
  \centering
  \includegraphics[width=1\linewidth]{sec/figure/more open-ended case wsi-vqa.pdf}
  \caption{Qualitative results on open-ended questions from the WSI-VQA dataset. The figure visualizes the Regions of Interest (RoIs) selected by PathAgent, along with the final predicted answer and the corresponding reasoning.}
  \label{fig:more open-ended case wsi-vqa}
\end{figure*}

\begin{table*}[t]
\caption{Comparison of zero-shot visual question answering between our PathAgent and current state-of-the-art methods on WSI-Bench and PathVQA datasets. The best performance is in \textbf{bold}, while the second-best performance is \underline{underlined}.}
    \centering
      \begin{tabular}{c|ccccc|c}
        \toprule
        \multirow{2}{*}{Method} & \multicolumn{5}{c|}{WSI-Bench} & PathVQA \\ 
        \cmidrule(lr){2-6} \cmidrule(lr){7-7}
        % \cline{3-7}
        & BLEU-1 &  BLEU-4 & ROUGE & METEOR & Accuracy & Accuracy \\ 
        \midrule
        Qwen3-VL~\cite{Qwen-VL} & 38.94 & 19.43 & 26.58 & 24.53 & 30.71 & 44.82 \\
        GPT-4o~\cite{GPT-4V} & 39.47 & 20.14 & 25.49 & 22.70 & 29.26 & 46.59 \\
        LLaVA-Med~\cite{llava-med} & 33.71 & 17.55 & 22.47 & 17.58 & 28.38 & 27.78 \\
        MedDr~\cite{meddr} & 34.63 & 18.66 & 23.71 & 20.39 & 28.24 & 29.35 \\
        Quilt-LLaVA~\cite{Quilt-llava} & 41.07 & 22.33 & 38.98 & 37.29 & 33.17 & 20.76 \\
        \midrule
        WSI-VQA~\cite{wsi-vqa} & 34.57 & 18.12 & 23.16 & 19.74 & 50.41 & 33.59 \\
        SlideChat~\cite{slidechat} & 44.25 & 21.36 & 42.09 & 41.38 & 55.48 & \underline{55.03} \\
        WSI-LLaVA~\cite{wsi-llava} & 46.71 & 23.49 & \textbf{46.47} & 45.29 & \underline{59.85} & 54.97 \\
        \textbf{PathAgent} & \textbf{48.92} & \textbf{24.51} & \underline{44.88} & \textbf{47.25} & \textbf{60.26} & \textbf{58.36}\\
        \bottomrule
      \end{tabular}%
    \label{tab:zero-shot on WSI-Bench and PathVQA}
\end{table*}

\begin{table*}
\caption{Ablation study on foundation models in PathAgent using Qwen3-4B as the Executor. The best performance is in \textbf{bold}, while the second-best performance is \underline{underlined}.}
    \centering
    \begin{tabular}{c|c|cccc|c}
        \toprule
        \multirow{2}{*}{Navigator} & \multirow{2}{*}{Perceptor} & \multicolumn{4}{c|}{WSI-VQA} &  SlideBench-VQA (BCNB) \\ 
        \cmidrule(lr){3-6} \cmidrule(lr){7-7}
        % \cline{3-7}
         & & BLEU-1 & BLEU-4 & METEOR & Accuracy & Accuracy \\ 
        \midrule
        \multicolumn{2}{c|}{WSI-VQA method} & 34.21 & 19.65 & 21.12 & 46.90 & 23.35 \\
        \midrule
        \multirow{3}{*}{PLIP} & Quilt-LLaVA & 44.53 & 43.46 & 25.03 & 52.95 & 49.33 \\
        & Patho-R1-3B & 48.17 & 46.79 & 29.61 & 53.67 & 51.43 \\
        \rowcolor{gray!20} &  Patho-R1-7B & \underline{52.89} & \underline{49.69} & \textbf{31.29} & \textbf{56.32} & \underline{54.72} \\
        \midrule
        \multirow{3}{*}{CPath-CLIP} & Quilt-LLaVA & 45.39 & 43.94 & 25.63 & 53.07 & 50.46 \\
        & Patho-R1-3B & 49.36 & 48.24 & 32.16 & 54.28 & 52.57 \\
        & Patho-R1-7B & \textbf{53.15} & \textbf{50.43} & \underline{30.59} & \underline{55.85} & \textbf{55.21} \\
        \bottomrule
      \end{tabular}
      \label{tab:ablation Navigator qwen3-4b}
\end{table*}

\begin{table*}
\caption{Ablation study of foundation models in PathAgent using Qwen3-32B as the Executor. The best performance is in \textbf{bold}, while the second-best performance is \underline{underlined}.}
    \centering
    \begin{tabular}{c|c|cccc|c}
        \toprule
        \multirow{2}{*}{Navigator} & \multirow{2}{*}{Perceptor} & \multicolumn{4}{c|}{WSI-VQA} &  SlideBench-VQA (BCNB) \\ 
        \cmidrule(lr){3-6} \cmidrule(lr){7-7}
        % \cline{3-7}
         & & BLEU-1 & BLEU-4 & METEOR & Accuracy & Accuracy \\ 
        \midrule
        \multicolumn{2}{c|}{WSI-VQA method} & 34.21 & 19.65 & 21.12 & 46.90 & 23.35 \\
        \midrule
        \multirow{3}{*}{PLIP} & Quilt-LLaVA & 45.35 & 44.41 & 25.70 & 51.58 & 50.47 \\
        & Patho-R1-3B & 52.46 & 50.47 & 31.50 & 54.77 & 53.26 \\
        &  Patho-R1-7B & \underline{55.58} & \underline{52.76} & \underline{34.10} & \underline{57.29} & \underline{55.02} \\
        \midrule
        \multirow{3}{*}{CPath-CLIP} & Quilt-LLaVA & 50.31 & 47.29 & 26.72 & 53.33 & 50.89 \\
        & Patho-R1-3B & 53.84 & 50.68 & 33.18 & 55.49 & 54.66 \\
        & Patho-R1-7B & \textbf{56.24} & \textbf{54.32} & \textbf{35.18} & \textbf{58.43} & \textbf{56.83} \\
        \bottomrule
      \end{tabular}
      \label{tab:ablation Navigator qwen3-32b}
\end{table*}

\section{Datasets Details}
\textbf{SlideBench-VQA~\cite{slidechat}.} The SlideBench-VQA dataset consists of two parts: SlideBench-VQA (TCGA) and SlideBench-VQA (BCNB). The questions are first cleaned using a large language model, and then screened by pathology experts according to inclusion criteria. SlideBench-VQA (TCGA) uses data from TCGA to construct 7,827 closed-set VQAs, with questions categorized into three main classes: Microscopy, Diagnosis, and Clinical, presenting a challenging dataset. The results are reported in accuracy. SlideBench-VQA (BCNB) is derived from the in-the-wild Early Breast Cancer Core-Needle Biopsy (BCNB) WSI dataset. It transforms the classification objective into a question format within a specific template, while converting the original multi-class labels into multiple-choice options. SlideBench-VQA (BCNB) comprises 7,247 closed-set VQA pairs from 1,058 patients, and the results are presented as accuracy. A specific modification in our evaluation is that we integrate the three receptor status questions of ER Type, PR Type and HER2 Type into Receptor Status for presentation.

\textbf{WSI-VQA~\cite{wsi-vqa}.} The WSI-VQA dataset contains a total of 977 WSIs with 8671 question-answering pairs derived from TCGA-BRCA. The dataset is constructed by leveraging TCGA’s diagnostic WSIs and associated clinical records, where a portion of the QA pairs are generated from slide-level captions using LLMs to produce multi-choice questions, while the remaining QA pairs are obtained from the clinical files in TCGA by extracting keywords to fit templates. Our zero-shot evaluation focuses on its test set, which contains 86 WSIs and 735 question-answering pairs. For the close-ended subset, accuracy is adopted by comparing the sentence similarity to measure the performance of the model. For the open-ended subset, BLEU~\cite{papineni2002bleu}, METEOR~\cite{banerjee2005meteor}, and ROUGE~\cite{lin2004rouge} are adopted for evaluation.

\textbf{PathMMU~\cite{pathmmu}.} The PathMMU dataset is a large-scale benchmark for evaluating large multi-modal models in computational pathology, comprising 33,428 multi-modal, multi-choice questions paired with 24,067 high-quality pathology images. All data underwent expert manual review to ensure clinical validity and professional quality. The questions are deliberately designed to demand fine-grained visual reasoning aligned with real diagnostic standards, rather than being solvable through textual cues alone, and the images maintain high clarity with an average resolution of approximately $900\times 700$ pixels. Our zero-shot evaluation focuses on the test set of PathMMU, where accuracy is adopted for evaluation. 

\textbf{WSI-Bench~\cite{wsi-llava}.} WSI-Bench is curated from TCGA and contains 10,756 WSIs across 30 cancer types, together with 179,569 VQA pairs. The training set consists of 175,450 VQA pairs (122,133 open-ended and 53,317 closed-ended) associated with 9,642 WSIs, while the testing set includes 4,119 VQA pairs (2,838 open-ended and 1,281 closed-ended) from 208 WSIs. Our zero-shot evaluation focuses on its morphological analysis and diagnosis subset, where accuracy is reported for closed-ended questions and BLEU, METEOR, and ROUGE are used for open-ended questions. To maintain task difficulty, the evaluated subset encompasses all 30 cancer types.

\textbf{PathVQA~\cite{pathvqa}.} The PathVQA dataset extracts pathological images and accompanying descriptions from textbooks and then generates question-and-answer pairs using natural language processing technology. The dataset collects 32,799 open-ended questions from 4,998 pathological images, and each question is manually reviewed to ensure accuracy. The accuracy of the yes-or-no question is be reported in our experiments.

\section{Experiment Details}
\subsection{Quantitative Evaluation on PathMMU}
As shown in \Cref{tab:zero-shot on PathMMU}, we present detailed results on the PathMMU dataset. Following the partitioning in ~\cite{pathmmu}, we report the accuracy on PubMed, SocialPath, EduContent, Atlas and PathCLS. On the RoI-level dataset, general-purpose Visual-language models (VLMs) like Qwen3-VL~\cite{Qwen-VL} and GPT-4o~\cite{GPT-4V} demonstrate capabilities comparable to well-trained WSI-specific models, achieving accuracies of 45.82\% and 49.31\%, respectively. Analysis on this type of dataset places lower demands on the model's diagnostic workflow planning capabilities compared to analyzing slide-level datasets, as the information in an image can be directly represented by a visual embedding.

The proposed PathAgent demonstrates state-of-the-art performance on the PathMMU dataset, particularly in the PathCLS class. In the PathCLS class, which encompasses widely recognized pathology classification datasets, PathAgent shows a significant performance improvement over other competing methods, specifically achieving a 19.25\% improvement over Quilt-LLaVA~\cite{Quilt-llava}, which achieves the second-highest accuracy in the PathCLS class.

% 我们展示了在PathMMU数据集中更详细的结果信息，遵循~\cite{Pathmmu}中的划分，我们报告了来自五类不同来源数据的Accuracy。在RoI-level的数据集上，general-purpose VLMs like Qwen3-VL and GPT-4o展示出了和well-trained WSI-specific models相媲美的能力，他们分别有着45.82和49.31的准确率。在这一类数据集上进行分析对模型诊断流程规划能力要求相对于slide-level的数据集低，因为图像信息可以由一个视觉特征嵌入表示，而非转换成多个patch视觉嵌入的堆叠。所提出的PathAgent在PathMMU数据集上展示出最优的性能，特别是对PathCLS类的分析。PathCLS类中包含widely recognized pathology classification datasets，在这一类中，PathAgent和其他对比方法有显著性能提升，即相对于具有第二高准确率的Quilt-LLaVA提高了19.25\%。

\begin{figure*}[t]
  \centering
  \includegraphics[width=0.86\linewidth]{sec/figure/more close-ended case wsi-vqa.pdf}
  \caption{Qualitative results on close-ended questions from the WSI-VQA dataset. The correct answers are highlighted in yellow.}
  \label{fig:more close-ended case wsi-vqa}
\end{figure*}

\begin{figure*}[t]
  \centering
  \includegraphics[width=1\linewidth]{sec/figure/more close-ended case slidechat.pdf}
  \caption{Qualitative results on close-ended questions from the SlideBench-VQA (TCGA) dataset. The correct answers are highlighted in yellow.}
  \label{fig:more close-ended case slidechat}
\end{figure*}

\subsection{Quantitative Evaluation on WSI-Bench and PathVQA}
\Cref{tab:zero-shot on WSI-Bench and PathVQA} shows the zero-shot visual question answering performance of current state-of-the-art methods and our PathAgent. On the WSI-Bench dataset, for Qwen3-VL, GPT-4o, LLaVA-Med, MedDR, and Quilt-LLaVA, considering that these models cannot directly process the entire WSI, we adjust the size of the WSIs to $1024 \times 1024$ and input them into the models. Experimental results show that using only thumbnails as substitutes for the entire WSI leads to a significant loss of accuracy, causing these models to perform worse than WSI-specific models (SlideChat and WSI-LLaVA) in zero-shot visual question answering. Furthermore, PathAgent achieves state-of-the-art results on almost all metrics, demonstrating the superiority of our method. On the PathVQA dataset, our method also achieves the best results, with an accuracy 3.33\% higher than that of the second-highest performing model, SlideChat.

% 在WSI-Bench数据集上，对于Qwen3-VL，GPT-4o，LLaVA-Med，MedDR和Quilt-LLaVA，考虑到这些模型不能直接处理整张WSI，我们adjusts the size of the WSI to 1024 × 1024 and inputs it into the model. 实验结果显示，仅使用thumbnail作为整张WSI的代替会导致精度的大量损失，导致这类模型在zero-shot visual question answering上的performance不如WSI-specific models (SlideChat and WSI-LLaVA) 性能好。此外，PathAgent在几乎所有指标上都取得了最优的成绩，这展现了本文方法的优越性。在PathVQA数据集上，我们的方法也取得了最优秀的结果，其准确率相比于第二高的SlideChat高出了3.33\%。

\subsection{Qualitative Evaluation on WSI-VQA}
In \Cref{fig:more close-ended case wsi-vqa}, we present the results of PathAgent on the WSI-VQA dataset for handling close-ended questions. PathAgent accurately assesses tumor status and analyzes disease progression. Specifically, the model demonstrates strong capabilities in identifying tumor size and determining pathological stage. Furthermore, PathAgent exhibits an understanding of microscopic morphology, correctly distinguishing between the intermediate nuclear grade and the Nottingham grade of invasive ductal carcinoma. Regarding clinical diagnostic details, PathAgent also performs surgical margin assessment and inference of immunohistochemical markers, demonstrating its ability to handle critical prognostic questions. Overall, PathAgent effectively analyzes WSIs, extracting key information to answer multi-scale questions ranging from the global to the local.
% 我们在\Cref{fig:more close-ended case wsi-vqa}中展示了PathAgent在WSI-VQA数据集上应对close-ended question的结果。PathAgent能够准确评估肿瘤的状态并分析疾病进展，具体来说，模型在识别肿瘤尺寸和判定病理分期上展现出强大能力。此外，PathAgent具备对微观形态学的理解，在区分Invasive ductal carcinoma的intermediate nuclear grade和nottingham grade时给出了正确的响应。在临床诊断细节方面，PathAgent也完成了手术边缘状态判断和免疫组化标记物的推断，表明其能够处理涉及预后的关键问题。总体来看，PathAgent能够有效分析WSI图像，从中提取关键信息以回答从整体到局部的多尺度问题。

Furthermore, in \Cref{fig:more open-ended case wsi-vqa}, we demonstrate PathAgent's ability to handle open-ended question answering and complex reasoning tasks. Unlike simple classification, these questions require the model to integrate features from WSIs, autonomously formulate an analysis plan, make logical pathological inferences, and provide interpretable justifications. In making predictions about a patient's vital status, PathAgent infers an ``alive'' status by identifying the presence of normal tissues and normal skin structures alongside potentially abnormal features, even without finding lethal visual evidence of malignancy. This demonstrates PathAgent's ability to correlate morphological features with clinical prognosis. In addition, PathAgent successfully completes the task of inferring the status of immunohistochemical markers from H\&E images. This type of highly challenging case will be further discussed in detail in \Cref{sec:challenging case}. For histological diagnoses, PathAgent also provides accurate diagnostic results and detailed pathological feature analyses. This ability to generate reasoning during the analysis process enhances the credibility and transparency of PathAgent's application in clinical diagnosis.
% 进一步地，我们在\Cref{fig:more open-ended case wsi-vqa}中展示了PathAgent处理开放式问答和复杂推理任务的能力。与简单的分类不同，这些问题要求模型整合WSI中的特征，自主制定分析计划，进行有逻辑的病理学推断，并给出可解释的依据。在回答关于患者vital status的预测时，PathAgent通过识别normal tissues和normal skin structures与potentially abnormal features的表现，在没有发现致死性恶性视觉证据的情况下推断出患者状态为alive，表明PathAgent具备将形态学特征和临床预后关联起来的能力。此外，PathAgent还完成了通过H&E染色图像中推断免疫组化标记物状态的任务，这一任务极具挑战性，针对这一类问题的细致解析会在\ref{sec:challenging case}中提及。对于组织学类型的诊断，PathAgent也能给出准确的诊断结果和详细的病理特征解析，这种在分析过程中生成Reasoning的能力增强了PathAgent应用于临床诊断的可信度和透明度。

\subsection{Qualitative Evaluation on SlideBench-VQA (TCGA)}
In \Cref{fig:more close-ended case slidechat}, we demonstrate PathAgent's comprehensive diagnostic capabilities on the SlideBench-VQA (TCGA) dataset. For the case on the left in the figure, PathAgent not only correctly diagnoses papillary adenocarcinoma but also accurately assesses its tumor grade and pathological stage. The case on the right in the figure showcases the model's accurate identification and analysis of specific histological subtype features. PathAgent accurately identifies infiltrating lobular carcinoma and points out the key feature of a single file line of cells in infiltrating lobular carcinoma. This demonstrates PathAgent's ability to handle complex clinical scenarios and its potential to construct complete case files from macroscopic to microscopic perspectives.
% 我们在\Cref{fig:more close-ended case slidechat}中展示了PathAgent在SlideBench-VQA (TCGA)数据集上进行综合诊断的能力。针对图中的左侧案例，PathAgent不仅正确诊断了Papillary adenocarcinoma，准确评估了其肿瘤分级和病理分期。图中右侧案例展现了模型对特定组织学亚型特征的准确识别和分析，PathAgent准确识别出Infiltrating lobular carcinoma，并指出了Infiltrating lobular carcinoma的Single file line of cells的关键特征。这表明PathAgent具备处理复杂临床场景的能力，具备从宏观到微观构建完整病例档案的潜力。

\subsection{Ablation Study on Foundation Models}
\Cref{tab:ablation Navigator qwen3-4b} and \Cref{tab:ablation Navigator qwen3-32b} present our ablation study on foundation models for the Navigator. As the capabilities of the foundation models improve, performance on both WSI-VQA and SlideBench-VQA (BCNB) datasets increases. Notably, the performance gap between using CPath-CLIP and PLIP as the Navigator is significantly wider when the Executor is equipped with Qwen3-32B compared to Qwen3-4B. This indicates that a more powerful Executor can better leverage the Navigator's advantages in retrieval, thereby obtaining more accurate RoIs to assist WSI analysis.

% \Cref{tab:ablation Navigator qwen3-4b} and \Cref{tab:ablation Navigator qwen3-32b}展示了我们针对Navigator进一步开展的Ablation study on foundation models，随着foundation models能力的提升，模型在WSI-VQA和SlideBench-VQA (BCNB)数据集上的表现也有提升。值得注意的是，针对Navigator在使用CPath-CLIP和PLIP之间的差距在Executor使用Qwen3-32B时要比Executor使用Qwen3-4B时差距要更大

\subsection{Analysis of the Challenging Case}\label{sec:challenging case}
As shown in \Cref{fig:error cases}, we detail the analysis workflow of PathAgent for a challenging case. In this case, PathAgent is asked to provide the HER2 status. During the diagnostic process, the Executor provides zoom-in guidance to obtain information on membranous staining intensity and the percentage of positive cells. Subsequently, the model examines morphological features such as nuclear atypia and a high nucleocytoplasmic ratio, predicting that the result of HER2 is positive. This result does not entirely align with the actual result, and the reason is also shown in the model's reasoning: for HER2 results, WSIs based solely on H\&E staining cannot provide a comprehensive picture; specific immunohistochemical testing is also required. In fact, a comprehensive assessment of HER2 status requires sequencing and protein information, meaning that the answers provided by relying solely on H\&E images have limitations. This suggests that future work could move towards aligning H\&E and immunohistochemical image information to address the problem of modality loss during analysis.
% 如\Cref{fig:error cases}所示，我们详细展示了PathAgent对一个具有挑战性的案例的分析流程。在这个案例中，PathAgent被要求给出the result of her2，在诊断流程中，the Executor给出放大指导以获取membranous staining intensity and percentage of positive cells的信息，随后模型检查到了核异型和高核质比的形态学特征，给出了Positive的预测。这与真实结果不完全一致，其原因也在zoom reason中展示了，即对于her2结果，仅根据H&E染色的WSI不能够给出全面的结果，还需要specific immunohistochemical testing。事实上，对HER2状态的全面评估还需要测序信息和蛋白质信息，这意味着仅使用HE图像回答问题所给出的答案存在局限性。暗示着未来的工作可以朝着HE图像和免疫组化图像信息对齐的方向发展，以应对分析过程中模态缺失的问题。

\begin{figure*}[t]
  \centering
  \includegraphics[width=0.89\linewidth]{sec/figure/error cases.pdf}
  \caption{Illustration of PathAgent analyzing a challenging case. PathAgent performs a zoom-in operation to derive the answer, providing a detailed explanation and the rationale for the zoom. The reason for model's inability to answer the question accurately is highlighted in yellow.}
  \label{fig:error cases}
\end{figure*}

\subsection{Analysis of Human Collaborative Experiment}
As shown in \Cref{fig:human operation details}, the descriptions generated by the Perceptor during the analysis process may focus on incorrect morphological characteristics. Pathologists can interrupt the analysis process at any time to correct these errors promptly. Ultimately, PathAgent can provide the correct answer and corresponding reasoning. Furthermore, when the RoIs selected by the Navigator are irrelevant the diagnostic targets required to answer the questions, pathologists can manually specify RoIs for PathAgent to analyze. PathAgent's ability to interact with pathologists and provide timely feedback demonstrates its strong potential for deployment in clinical scenarios.

% 如\Cref{fig:human operation details}所示，PathAgent在分析过程中生成的描述存在问题，pathologists可以随时打断分析进程，对错误的描述进行修正，以及时纠正错误，最终PathAgent能够给出正确答案和相应的Reason。此外，当PathAgent选取的RoIs和实际回答问题需要关注的区域不相关时，pathologists可以指定RoIs，让PathAgent开展后续分析。PathAgent能和pathologists进行实时交互并及时给出交互反馈，展现出PathAgent具备部署于临床场景中的强大潜力。

% \begin{figure*}[t]
%   \centering
%   \includegraphics[width=0.89\linewidth]{sec/figure/prompt qwen.pdf}
%   \caption{The prompt used to execute Multi-Step Reasoning process in the Executor.}
% \end{figure*}

% \begin{figure*}[t]
%   \centering
%   \includegraphics[width=0.89\linewidth]{sec/figure/prompt vlm.pdf}
%   \caption{The prompt used to generate descriptions for the patches in Quilt-LLaVA and Patho-R1.}
% \end{figure*}

\begin{figure*}[t]
  \centering
  \includegraphics[width=0.84\textwidth]{sec/figure/human operation details.pdf}
  \caption{Illustration of how pathologists interact with PathAgent to select RoIs and check visual evidence. The correct answers are highlighted in yellow. Errors made by PathAgent during the analysis process are highlighted in red, whereas both corrections provided by pathologists and PathAgent's subsequent responses are highlighted in green.}
  \label{fig:human operation details}
\end{figure*}

\section{Prompt}

\subsection{Multi-Step Reasoning Prompts in the Executor} 
To execute Multi-Step Reasoning process, the following prompts are used:
\begin{itemize}
    \item Predict Answer: You are an expert AI pathology assistant. Your task is trying to answer the question step-by-step based on the patch descriptions. Output ONLY a JSON object: \{``answer'': ``the final predicted answer (string)'', ``thinking\_steps'': ``your detailed reasoning, step-by-step (string)''\}.
    \item Self Reflect: You are an expert AI pathology assistant. Your task is to judge whether the current patch descriptions are sufficient to confidently support the answer. Output ONLY a JSON object: \{``sufficient'': ``Yes'' or ``No''\}.
    \item Explore Missing Information: You are an expert AI pathology assistant. Your task is to specify what visual evidence is missing and whether zooming in could help obtain that evidence. Output ONLY a JSON object: \{``missing\_info'': ``noun phrase'', ``zoom\_recommendation'': ``Yes'' or ``No'', ``recommended\_zoom\_level'': ``None'' or an integer like 10 or 20 or 40, ``zoom\_reason'': ``brief reason why zooming helps''\}.
\end{itemize}

\subsection{Final Answer Generation Prompts in the Executor}
To generate the final answer based on the analytic states from all the iterations, the following prompts are used:
\begin{itemize}
    \item You are an expert slide-level pathology assistant. You will be given a question and detailed patch-level descriptions of a pathology slide. Your task is to infer the specific slide-level diagnostic result based on the provided evidence — not to define or explain the medical term itself. The answer should directly reflect the information observable in the slide, such as biomarker expression level, presence or absence of features, or a numeric measurement.
\end{itemize}

\subsection{Patch Descriptions Generation Prompts in the Perceptor} 
To generate descriptions for the patches, the following prompts are used:
\begin{itemize}
    \item Quilt-LLaVA: A conversation between a curious user and an AI medical assistant specialized in pathology image analysis. The assistant can interpret pathology images, describe observed features, and provide possible explanations based on medical knowledge, but will never give a definitive diagnosis or prescribe treatment. The assistant must always maintain a polite, clear, and professional tone. All answers should be supported by established, reliable medical sources. The assistant should carefully consider visual details in pathology images, such as cell morphology, staining patterns, and tissue architecture.
    \item Patho-R1: A conversation between a curious user and an AI medical assistant specialized in pathology image analysis. The assistant can interpret pathology images, describe observed features, and provide possible explanations based on medical knowledge, but will never give a definitive diagnosis or prescribe treatment. The assistant must always maintain a polite, clear, and professional tone. All answers should be supported by established, reliable medical sources. The assistant should carefully consider visual details in pathology images, such as cell morphology, staining patterns, and tissue architecture.
\end{itemize}
